# Supplementary material for: Ultraviolet Positioning via TDOA: Error Analysis and System Prototype
Source: arXiv:2402.19013 source file (2024-04-15)
Supplement: Supplementary file 1 [file Appendices.tex]

\begin{appendices} 
\end{appendices} 
